# Supplementary material for: Matrix-free construction of HSS representation using adaptive randomized sampling
Source: arXiv:1810.04125 source file (2018-10-11)
Supplement: Supplementary file 1 [file appendix_communication.tex]

%%%%%%%%%%%%%%%%%%%%%%%%%%%%%%%%%%%%%%%%%%%%%%%%%%%%%%%%%%%%%%%%%%%%%%%%
%%% Appendix for Communication analysis

\begin{center}
    \huge\textbf{Communication analysis \\(along the critical path)}
\end{center}

\begin{flushleft}
    \begin{equation*}
    [ \# \mbox{messages} \cdot \mbox{volume} ] \approx f \left( \mbox{latency} \cdot \frac{1}{\mbox{bandwidth}} \right) \propto (\alpha, \frac{1}{\beta})
    \end{equation*}
\end{flushleft}

% % % % % % % % % % % % % % % % % % % % % % % % % % % % % % % % % % % % % % % % % % % % % 
% Defining vocabulary
% % % % % % % % % % % % % % % % % % % % % % % % % % % % % % % % % % % % % % % % % % % % % 

Point-to-point: $ \alpha + \omega \cdot \beta ~~~~~~~~~~~~~~~~~~~~~~~~~~~~~~~~~~~ [1, w]$

Beast of $w$ words: $ \alpha \cdot \log(p) + \omega \cdot \log(p) ~~~~~ \log(p) \cdot [1, w]$

\section{ScaLAPACK}

Communciation: $\left[ C_m \frac{N}{\NB}, C_v \frac{N^2}{\sqrt{p}}\right]$

\noindent
$C_m = \log_2{p}$: Need to broadcast a message at each panel. \\
$C_v = \log_2{p}$: Each element is sent to $\sqrt{p}$ processors.

\section{PxGEMM}
Pipelined SUMMA (No $\log(p)$ term)

It multiplies two matrices of sizes: $M \times K, K \times N$

Generalization: not to communicate the largest matrix.

Three cases:
\begin{itemize}
\item $M,N \gg K$, communicate $A,B$.
\item $K,N \gg M$, communicate $A,C$.
\item $M,K \gg N$, communicate $B,C$.
\end{itemize}

In our case: $S = A \cdot R. A \gg R,S$, then communicate $R,S$. \\

Cost: \textcolor{blue}{$[r, \frac{r \cdot m}{\sqrt{p}}]$} \\

\textbf{Redistribution [Prylli and Tourancheau 1997, PxGEMMR2R]}

$n \times n$ block form: $P_1$-grid to $P_2$-grid.

Sender: \textcolor{blue}{$[P_2, \frac{n^2}{P_1}]$}

Receiver: \textcolor{blue}{$[P_1, \frac{n^2}{P_2}]$}

% % % % % % % % % % % % % % % % % % % % % % % % % % % % % % % % % % % % % % % % % % % % % 
% Original algorithm (old)
% % % % % % % % % % % % % % % % % % % % % % % % % % % % % % % % % % % % % % % % % % % % % 
\newpage
\section{Original algorithm (old)}

Assume: final rank $r$, and $p$ processors at current ``pc'' mode. Doubling strategy. \\

Steps: \textcolor{blue}{$s = \log{\frac{r}{d_0}}$} \\

Each ID (QR) has size: \textcolor{blue}{$m \cdot ( d_0 \cdot 2^i)$} \\

Cost: \textcolor{blue}{ $\log(p) \cdot \left[ \frac{d_0 \cdot 2^i}{\NB},\frac{m \cdot (d_0 \cdot 2^i)}{\sqrt{p}} \right].$ } \\

All ID:

\begin{equation*}
\begin{split}
\sum_{i=0}^{s} = \log(p) \cdot \left[ \frac{d_0 \cdot 2^i}{\NB},\frac{m \cdot (d_0 \cdot 2^i)}{\sqrt{p}} \right] = 
\log(p) \cdot \left[ \frac{d_0 }{\NB} \sum_{i=0}^{s} 2^i, \frac{m \cdot d_0}{\sqrt{p}} \sum_{i=0}^{s} 2^i \right] = 
\log(p) \cdot \left[ \frac{d_0 }{\NB} 2^{s+1}, \frac{m \cdot d_0}{\sqrt{p}} \sum_{i=0}^{s} 2^{s+1} \right] = \\
\textcolor{blue}{\log(p) \cdot \left[ \frac{2r}{\NB} , \frac{2r \cdot m}{\sqrt{p}} \right]}.
\end{split}
\end{equation*} \\

Redistribution from descendants to the node ``pc''. \\

Each restart: From direct child: size: $ \frac{m}{2} \cdot \Delta d$

$$ \Delta d = d_0 (2^i-2^{i-1}) = d_0 \cdot 2^{i-1} $$

Receiver: \textcolor{blue}{ $ \left[ \frac{p}{2}, \frac{ \frac{m}{2} \cdot d_0 2^{i-1} }{p} \right] $. }\\

Sender: \textcolor{blue}{ $ \left[ p, \frac{ \frac{m}{2} \cdot d_0 2^{i-1} }{ p/2 } \right] $. }\\

Adding all levels ( $p,\frac{p}{2},\frac{p}{4},..., L$). $m$ is halved at each level: \\

\textcolor{blue}{ $ \left[ 2p, \frac{m \cdot d_0 2^{i-1} }{p} \cdot L\right] $. } \\

Adding all restarts:

$$ s = \log(\frac{r}{d_0}) $$

\begin{equation*}
\sum_{i=1}^{s} = \left[ 2p ,\frac{m \cdot d_0 \cdot 2^i }{p} \cdot L \right] = 
\left[ 2p \cdot s , \frac{m \cdot 2r }{p} \cdot L \right] = 
\textcolor{blue}{\left[ 2p \log( \frac{r}{d_0}) , \frac{m \cdot 2r }{p} \cdot L \right].}
\end{equation*} \\

% % % % % % % % % % % % % % % % % % % % % % % % % % % % % % % % % % % % % % % % % % % % % 
% Stable algorithm (latest)
% % % % % % % % % % % % % % % % % % % % % % % % % % % % % % % % % % % % % % % % % % % % % 
\newpage
\section{Stable algorithm (latest)}
\noindent

Each QR size: $m \cdot \Delta d$ \\

Interpolative decomposition cost: $\IDCost$ \\

Orthogonalization: 2 GEMM\\

$Q_{i3} = S_{i3} - Q_{i1ui2} (Q_{i1ui2})^* S_{i3}$ \\

Costs ( $d = \Delta d \cdot i$ ):

$$ 1)~~~ [ \Delta d,\frac{\Delta d \cdot (m+d)}{\sqrt{p}} ] $$
$$ 2)~~~ [ \Delta d,\frac{\Delta d \cdot (m+d)}{\sqrt{p}} ] $$

Number of steps: $s = \frac{r}{\Delta d}$ \\

All QR:

\begin{equation*}
\sum_{i=1}^{s} \IDCost = \textcolor{blue}{ \log(p) \cdot \left[ \frac{r}{\NB},\frac{m \cdot r}{\sqrt{p}} \right]. }
\end{equation*} \\

All Orthogonalization:

\begin{equation*}
2 \cdot 2 \cdot \sum_{i=1}^{s} \left[ \Delta d , \frac{ \Delta d (m+d)}{\sqrt{p}}  \right] = 
4 \cdot \left[ r, \sum_{i=1}^{s} \frac{m+{\Delta d}^2 \cdot i}{\sqrt{p}} \right] = 
\textcolor{blue}{ 4 \cdot \left[ r, \frac{mr+r^2/2}{\sqrt{p}} \right]. }
\nonumber
\end{equation*}

Redistribution \\

Each restart: 

Direct child size $ \frac{m}{2} \cdot \Delta d$ \\

Receiver: $ \left[ \frac{p}{2}, \frac{ \frac{m}{2} \cdot \Delta d}{p} \right] $. \\
Sender: $ \left[ p, \frac{ \frac{m}{2} \cdot \Delta d}{ p/2 } \right] $. \\

All levels: $ \left[ 2p, L \cdot \frac{m \cdot \Delta d }{p} \right] $. \\

All restarts: 
\begin{equation*}
    \sum_{i=1}^{s} \left[ 2p , L \cdot \frac{m \cdot \Delta d }{p} \right] = 
    \textcolor{blue}{ \left[ 2p \cdot \frac{r}{\Delta d}, L \cdot \frac{m \cdot r }{p} \right]. }
\end{equation*}
